# Supplementary material for: The Baum-Connes conjecture, Swan group actions and controlled topology
Source: arXiv:1303.0701 source file (2013-03-04)
Supplement: Supplementary file 1 [file appendix.tex]

\begin{appendix}

\section*{Appendix}
\section{$C^{*}$-algebras and continuous function calculus}

This section is a short reminder of the definition of the continuous function calculus on a $C^{*}$-algebra. \\

\begin{definition}
For a commutative $C^{*}$-algebra $A$, let $Sp(A)$ be the set of algebra homomorphisms from $A$ to $\IC$. We view $Sp(A)$ as a subspace of the space of linear functionals $A \rightarrow \IC$, equipped with the weak-$^{*}$-topology.
\end{definition}

\fxnote{define U(A) and GL(A) for nonunital algebras}

\begin{prop}
\label{unitaryvsinvertible}
Let $A$ be a $C^{*}-algebra$. Then $U(A)$ is a deformation retract of $GL(A)$.
\end{prop}

\begin{proof}
Let us first consider the case where $A$ already is unital. Then $U(A)$ and $GL(A)$ are just the unitaries respectively invertibles in $A$. Let $x$ be invertible. Then %find source
\end{proof}

\pagebreak
\section{Hilbert Modules}

\begin{example}
Let $A$ be a $C^{*}$-algebra and $a_{1}, a_{2}, \cdots$ a sequence of elements of norm $1$. Then the matrix
\[
\begin{pmatrix}
a_{1} \\
a_{2} \\
a_{3} \\
\cdots
\end{pmatrix}
\]
never represents a bounded operator from $A$ to $\oplus_{\IN} A$. However, its potential adjoint
\[
\begin{pmatrix}
a_{1} & a_{2} & a_{3} & \cdots
\end{pmatrix}
\]
may represent a bounded operator. For example, if $A = C[0,1]$, let $a_{i}$ be a continuous function supported on $[\frac{1}{i+1}, \frac{1}{i}]$ with norm $1$. Then we estimate for the corresponding operator $T: \oplus_{\IN} A \rightarrow A$
\begin{align*}
\left\Vert T(\sum\limits_{\IN} b_{i} e_{i}) \right\Vert^{2} 
&= \left\Vert \sum\limits_{\IN} b_{i} a_{i}  \right\Vert^{2} \\
&= \sup_{i} \left\Vert b_{i} \right\Vert^{2} \\
&\leq \left\Vert \sum\limits_{\IN} b_{i}b_{i}^{*} \right\Vert \\
&= \left\Vert \sum\limits_{\IN} b_{i}e_{i} \right\Vert
\end{align*}
and hence $T$ is bounded. \fxnote{Check.}
\end{example}

\pagebreak
\section{Crossed products}

This section collects some definitions and facts about twisted group rings and reduced crossed products. 

\begin{definition}
Let $A$ be a ring with a left $G$-action, which we will denote by $(a,g) \mapsto g(a)$. The twisted group ring or crossed product of $A$ and $G$ $A \rtimes G$ is the ring with elements formal finite sums $\sum\limits_{i} a_{i} g_{i}$ with $g_{i} \in G, a_{i} \in A$. Multiplication is defined by setting
\[
ag \cdot bh = a g(b) gh
\]
and extending $\IZ$-bilinearly. It is easy to check that this multiplication is associative.
\end{definition}

\begin{rem}
Analogously, we can define a twisted group ring $G \rtimes A$ if $A$ has a right $G$-action. Its elements are of the form $\sum\limits_{i} g_{i}a_{i}$, and multiplication is defined such that
\[
ga \cdot hb = gh a^{h}b
\]
Regarding a ring with right $G$-action as a ring with left $G$-action by letting $g$ act as $g^{-1}$ from the right, we can form two twisted group rings $A \rtimes G$ and $G \rtimes A$. The map sending $ga \in A \rtimes G$ to $g(a) g = (a^{g^{-1}}) g \in G \rtimes A$ is an isomorphism between these two rings.
\end{rem}

\begin{prop}
\label{covariant}
Let $M$ be a left $A$-module. A left $A \rtimes G$-module structure is then the same as a left $G$-action on $M$, $(m,g) \mapsto g(m)$ such that
\[
g(ma) = g(m)g(a)
\]
We call a pair consisting of the left actions of $A$ and $G$ satisfying this condition a covariant representation of $(A,G)$.
\end{prop}

\begin{proof}
For $ag \in G \rtimes A$, we define
\[
ag \cdot m = ag(m)
\]
and extend linearly. The only thing to check is that
\[
bh \cdot (ag \cdot m) = (bh \cdot ag) \cdot m 
\]
for $g,h \in G, a, b \in A$. The left-hand side computes to $b h(ag(m))$ and the right-hand side to $bh(a) (hg)(m)$. The assumption guarantees that this is the same.
\end{proof}

If $A$ comes with an involution and $G$ acts involution-preserving on $A$, we can define an involution on $G \rtimes A$ via
\[
(ag)^{*} = g^{-1}(a^{*}) g^{-1}
\]
It is straightforward to check that this involution is anti-multiplicative. 

\subsection{Reduced Group $C^{*}$-algebras}

Now assume $A$ is a $C^{*}$-algebra with an involution-preserving right $G$-action. 

\begin{definition}
Let $l^{2}(G,A)$ be the complete Hilbert $A$-module with basis $G$. We define a left $G$-action $\rho$ on $l^{2}(G,A)$ via
\[
\rho(g)(\sum a_{i}g_{i}) = \sum a_{i} gg_{i}
\]
and a left module action $\tau$ of $A$ on $l^{2}(G,A)$ via
\[
\tau(a)(\sum a_{i}g_{i}) = \sum g_{i}^{-1}(a)a_{i} g_{i}
\]
This is a covariant representation of $(A,G)$, called the regular representation, compare \cite[Def. 2.20]{HG}.
\end{definition}

\pagebreak
\section{$C^*$-categories and $L$-theory}

\subsection{$C^*$-algebras and symmetric forms}

The following theorem classifies symmetric forms over $C^*$-algebras; compare \cite{analyticnovikov}[1.6].

\begin{thm}
\label{forms}
Let $A$ be a $C^*$-algebra with unit and let $(A^n,p)$ be a projective module defined by a projection $p$. Let $\phi: (A^n,p) \rightarrow (A^n,p)$ be a symmetric form, i.e. a selfadjoint invertible. Then there are projections $p_+$ and $p_-$ in $A^n$ with $(A^n,p_+) \oplus (A^n,p_-) \cong (A^n,p)$ such that $\phi$ is isometric to the form $1 \oplus -1$ on $(A^n,p_+) \oplus (A^n,p_-)$, and this decomposition is unique up to isomorphism.
\end{thm}

\begin{proof}
We may assume that $\phi: A \rightarrow A$ by replacing $A$ with $\End(A^n,p)$ if necessary. If $\phi$ is positive, $\phi^{\frac{1}{2}}$ defines an isometry from $\phi$ to $1$; similarly if $\phi$ is negative, $(-\phi)^{1/2}$ defines an isometry from $\phi$ to $-1$. In general, since $\phi$ is invertible, its spectrum has a gap around $0$. Let $f_+$ be a continuous function which is $1$ on the positive part of the spectrum and $0$ on the negative part; $p_+ = f_+(\phi)$ is called the \emph{positive projection} of $\phi$. Similarly, using a function $f_-$ which is $1$ on the negative part of the spectrum and $0$ on the positive part, one defines a projection $p_-$, called the \emph{negative projection} of $\phi$.  Note that $p_+ + p_1 = 1$, hence $A \cong (A.p_+) \oplus (A,p_-)$. This splitting is $\phi$-invariant since $\phi$ commutes with both $p_+$ and $p_-$. Furthermore, $ap_+\phi = ap_+(p_+\phi)$, hence $\phi$ is given by the positive element $p_+\phi$ on $(A,p_+)$ and similarly by the negative element $p_-\phi$ on $(A,p_-)$. Hence $\phi$ decomposes as a direct sum of one negative and one positive symmetric, and we have already seen that a positive symmetric form is isometric to $1$ and a negative form is isometric to $-1$.  This proves the existence part.  \\
Proving uniqueness is unfortunately quite a mess. We have to see that, given 4 projective modules $P_1, P_2, Q_1, Q_2$ and an isometry $k$ between the two forms $1 \oplus -1: P_1 \oplus P_2$ and $1 \oplus -1: Q_1 \oplus Q_2$, $P_1$ and $Q_1$ and $P_2$ and $Q_2$ are isomorphic. Writing $k$ as a $2 \times 2$-matrix $(k_{ij})$ and writing out what it means to be an isometry between the two forms, we find that $k_{11}k_{11}^* = 1+k_{12}k_{12}^*$ and, by considering $k^*$ as an isometry in the other direction, $k_{11}^*k_{11} = 1+k_{12}^*k_{12}$ and hence $k_{11}^*k_{11}$ and $k_{11}k_{11}^*$ are both invertible. It follows that $k_{11}$ is invertible since it has both a right and a left inverse. The same argument applies to $k_{22}$.
\end{proof}

We also record a kind of "homotopy invariance" of symmetric forms:

\begin{prop}
\label{homotopy}
Let $\phi$ and $\psi$ be symmetric forms in a $C^*$-algebra $A$. Assume that $\phi$ and $\psi$ are connected by a path of selfadjoint invertibles.. Then $\phi$ and $\psi$ are isometric. By considering the linear path from $\phi$ to $\psi$, this is in particular the case if $\psi$ lies inside some open ball around $\phi$ consisting only of invertibles.
\end{prop}

\begin{proof}
Let $\gamma$ be such a path from $\phi$ to $\psi$. The process of forming the positive and negative projections of $\gamma(t)$ depends continuously on $t$, hence $\phi_+$ and $\psi_+$ are connected by a path of projections which implies that $\phi_+$ and $\psi_+$ are unitarily equivalent. The same argument applies to the negative projections, hence the proposition follows.
\end{proof}

Now that we know that isometry classes of symmetric forms on projective modules over a $C^*$-algebra correspond to pairs of isomorphism classes of projective modules, it is easy to deduce what $L_0^p$ of a $C^*$-algebra is:

\begin{prop}
The functors $K_0^{top}$ and $L_0^p$ on the category of $C^*$-algebras are naturally isomorphic.
\end{prop}

\begin{proof}
Isometry classes of symmetric forms correspond to pairs of projective modules; since 2 is invertible, dividing out hyperbolic forms corresponds to dividing out the pairs $(P,P)$ for any projective module $P$. The result is clearly $K_0^{top}$.
\end{proof}

\subsection{$C^*$-algebras and symmetric forms}

The following theorem classifies symmetric forms over $C^*$-algebras; compare \cite[1.6]{analyticnovikov}.

\begin{thm}
\label{forms}
Let $A$ be a $C^*$-algebra with unit and let $(A^n,p)$ be a projective module defined by a projection $p$. Let $\phi: (A^n,p) \rightarrow (A^n,p)$ be a symmetric form, i.e. a selfadjoint invertible. Then there are projections $p_+$ and $p_-$ in $A^n$ with $(A^n,p_+) \oplus (A^n,p_-) \cong (A^n,p)$ such that $\phi$ is isometric to the form $1 \oplus -1$ on $(A^n,p_+) \oplus (A^n,p_-)$, and this decomposition is unique up to isomorphism.
\end{thm}

\begin{proof}
We may assume that $\phi: A \rightarrow A$ by replacing $A$ with $\End(A^n,p)$ if necessary. If $\phi$ is positive, $\phi^{\frac{1}{2}}$ defines an isometry from $\phi$ to $1$; similarly if $\phi$ is negative, $(-\phi)^{1/2}$ defines an isometry from $\phi$ to $-1$. In general, since $\phi$ is invertible, its spectrum has a gap around $0$. Let $f_+$ be a continuous function which is $1$ on the positive part of the spectrum and $0$ on the negative part; $p_+ = f_+(\phi)$ is called the \emph{positive projection} of $\phi$. Similarly, using a function $f_-$ which is $1$ on the negative part of the spectrum and $0$ on the positive part, one defines a projection $p_-$, called the \emph{negative projection} of $\phi$.  Note that $p_+ + p_1 = 1$, hence $A \cong (A.p_+) \oplus (A,p_-)$. This splitting is $\phi$-invariant since $\phi$ commutes with both $p_+$ and $p_-$. Furthermore, $ap_+\phi = ap_+(p_+\phi)$, hence $\phi$ is given by the positive element $p_+\phi$ on $(A,p_+)$ and similarly by the negative element $p_-\phi$ on $(A,p_-)$. Hence $\phi$ decomposes as a direct sum of one negative and one positive symmetric, and we have already seen that a positive symmetric form is isometric to $1$ and a negative form is isometric to $-1$.  This proves the existence part.  \\
Proving uniqueness is unfortunately quite a mess. We have to see that, given 4 projective modules $P_1, P_2, Q_1, Q_2$ and an isometry $k$ between the two forms $1 \oplus -1: P_1 \oplus P_2$ and $1 \oplus -1: Q_1 \oplus Q_2$, $P_1$ and $Q_1$ and $P_2$ and $Q_2$ are isomorphic. Writing $k$ as a $2 \times 2$-matrix $(k_{ij})$ and writing out what it means to be an isometry between the two forms, we find that $k_{11}k_{11}^* = 1+k_{12}k_{12}^*$ and, by considering $k^*$ as an isometry in the other direction, $k_{11}^*k_{11} = 1+k_{12}^*k_{12}$ and hence $k_{11}^*k_{11}$ and $k_{11}k_{11}^*$ are both invertible. It follows that $k_{11}$ is invertible since it has both a right and a left inverse. The same argument applies to $k_{22}$.
\end{proof}

For later uses, we also record a kind of "homotopy invariance" of symmetric forms:

\begin{prop}
\label{homotopy}
Let $\phi$ and $\psi$ be symmetric forms in a $C^*$-algebra $A$. Assume that $\phi$ and $\psi$ are connected by a path of selfadjoint invertibles.. Then $\phi$ and $\psi$ are isometric. By considering the linear path from $\phi$ to $\psi$, this is in particular the case if $\psi$ lies inside some open ball around $\phi$ consisting only of invertibles.
\end{prop}

\begin{proof}
Let $\gamma$ be such a path from $\phi$ to $\psi$. The process of forming the positive and negative projections of $\gamma(t)$ depends continuously on $t$, hence $\phi_+$ and $\psi_+$ are connected by a path of projections which implies that $\phi_+$ and $\psi_+$ are unitarily equivalent. The same argument applies to the negative projections, hence the proposition follows.
\end{proof}

Now that we know that isometry classes of symmetric forms on projective modules over a $C^*$-algebra correspond to pairs of isomorphism classes of projective modules, it is easy to deduce what $L_0^p$ of a $C^*$-algebra is:

\begin{prop}
The functors $K_0^{top}$ and $L_0^p$ on the category of $C^*$-algebras are naturally isomorphic.
\end{prop}

\begin{proof}
Isometry classes of symmetric forms correspond to pairs of projective modules; since 2 is invertible, dividing out hyperbolic forms corresponds to dividing out the pairs $(P,P)$ for any projective module $P$. The result is clearly $K_0^{top}$.
\end{proof}

The above proposition carries over to $C^*$-categories with virtually the same proof:

\begin{prop}
The functors $L_0^p$ and $K_0^{top}$ on the category of $C^*$-categories are naturally isomorphic. 
\end{prop}

\begin{proof}
Let $\phi: (A,p) \rightarrow (A,p)$ be a symmetric form. By applying \ref{forms} to the $C^*$-algebra $\End((A,p))$, we obtain projective modules $(A,p_+)$ and $(A,p_-)$ such that $\phi$ is isometric to $1 \oplus -1$ on $(A,p_+) \oplus (A,p_-)$. As above, the map $L_0^p(\C) \rightarrow K^{top}(\C), [\phi] \rightarrow p_+-p_-$, is an isomorphism.
\end{proof}

\begin{prop}
For any $C^*$-category $\C$, multiplication by $2$ annihilates both the kernel and the cokernel of the natural map $i: L_0(\C) \rightarrow L_0^p{\C}$. 
\end{prop}

\begin{proof}
This is a consequence of the Rothenberg sequence. However, since we understand symmetric forms in $C^*$-categories, we can give an explicit proof, compare \cite{analyticnovikov}[1.7]. \\
Let $\tilde{K_0}(\C)$ be the cokernel of the inclusion $K_0^{alg}(A) \rightarrow K_0^{alg}(\Idem(A))$. It easily follows from the classification of forms that $L_0(\C)$ is the group
\[
\{(P,Q) \in K_0(\Idem(\C)) \times K_0(\Idem(\C)): P+Q = 0 \in \tilde{K_0}(\C) \} / <\{(A,A): A \in \C\}>
\]

The kernel of $i$ is given by pairs $(P,P)$ in $K_0^p(\C)$ with $2P = 0$ in $\tilde{K_0}(\C)$. We may change $(P,P)$ by adding or subtracting $(A,A)$ for $A$ an actual object of $\C$ without changing the $L_0$-class $(P,P)$ represents. This means that the $L_0$-class $(P,P)$ represents only depends on $P \in \tilde{K_0}(\C)$, and hence the kernel identifies with the $2$-torsion in $\tilde{K_0}(\C)$. \\
For the cokernel, clearly $i$ hits $K_0^{alg}(\C) \subset K_0^{top}(\C) \cong L_0^p(\C)$. Hence to compute the cokernel, we may interpret $i$ as a map from $L_0(\C)$ to $\tilde{K_0}(\C)$. The image consists of the differences $P-Q$ such that $P+Q = 0$, i.e. of the elements of the form $2P$. So the cokernel is $\tilde{K_0}(\C)/2\tilde{K_0}(\C)$.
\end{proof}

\pagebreak
\section{Cohomology of groups}

This is a short review of group cohomology, with an emphasis on the relation between group cohomology and group extensions. The main source for the following is \cite{brown}. 

\fxnote{derived functor}

\subsection{The Bar resolution}

For the rather explicit computations we want to use group cohomology for, we have to introduce one special resolution of $\IZ$ as $\IZ G$-module, the so-called Bar resolution.

\begin{definition}
Let $F_{n}$ be the free $\IZ$-module generated by all $n+1$-tuples $(g_{0}, g_{1}, \cdots g_{n})$ of elements of $G$.  The group $G$ acts on $F_{n}$ via
\[
g \cdot (g_{0}, \cdots g_{n}) = (gg_{0}, \cdots gg_{n})
\]
Let $d_{i}: F_{n} \rightarrow$ for $0 \leq i \leq n$ be defined as
\[
d_{i}(g_{0}, g_{1}, \cdots g_{i}, \cdots g_{n}) = (g_{0}, g_{1}, \cdots \hat{g_{i}}, \cdots g_{n}) 
\]
where $\hat{}$ means that we omit $g_{i}$. Define $\partial: F_{n} \rightarrow F_{n-1}$ as $\partial = \sum\limits_{i=0}^{n} (-1)^{i} d_{i}$. Define the agumentation $ \epsilon: F_{0} \rightarrow F_{-1} = \IZ$ as $\epsilon(g_{0}) = 1$ for each $g_{0} \in G$. 
\end{definition}

\begin{prop}
The $F_{i}$ form a free resolution of $\IZ$ by $\IZ G$-modules, called the Bar resolution and denoted by $F$.
\end{prop}

\begin{proof}
It is straightforward to check that $F_{n}$ together with the augmentation is a chain complex. The elements of the form $(1,g_{1}, \cdots g_{n})$ form a basis of $F_{n}$ as $\IZ G$-module, hence $F_{n}$ is a free $\IZ G$-module. It remains to see that the complex $F_{i}$ is acyclic. A chain contraction is defined by
\[
h(g_{0}, \cdots g_{n}) = (1,g_{0}, \cdots g_{n})
\]
if $n \geq 0$ and $h(1) = 1$ for $n = -1$. It is straightforward to check that this is indeed a chain contraction.	
\end{proof}

Frequently, the $\IZ G$-basis elements $(1,g_{1},\cdots g_{n})$ of $F_{n}$ are written in the bar notation, where $[g_{1} \mid g_{2} \mid \cdots \mid g_{n}] $ in the bar notation corresponds to the basis element $(1,g_{1}, g_{1}g_{2}, \cdots g_{1}g_{2}\cdots g_{n})$ of $F_{n}$. The $d_{i}$ then take the form
\[
d_{i}([g_{1} \mid g_{2} \mid \cdots \mid g_{n}] ) = \begin{cases}
g_{1} [g_{2} \mid \cdots \mid g_{n}] &\text{ if } i = 0 \\
[g_{1} \mid g_{2} \mid \cdots g_{i-1} \mid  g_{i}g_{i+1} \mid g_{i+2} \cdots \mid g_{n}] &\text{ if } 0 < i <n \\
[g_{1} \mid g_{2} \mid \cdots \mid g_{n-1}]  &\text{ if } i = n
\end{cases}
\]

If $M$ is a $G$-module, the homology of the complex $\Hom_{\IZ G}(F,M)$ is the group cohomology of $G$ with coefficients in $M$. 

\fxnote{Functoriality}
\fxnote{Normalized Bar complex}

\subsection{$H^{2}$ and group extensions}

Given an abelian group $A$ and a group $F$, we will give the relationship between group cohomology and the classification of all extensions of the form
\[
0 \rightarrow A \rightarrow G \rightarrow F \rightarrow 0
\]
up to isomorphisms of the form
\[
\xymatrix{
0 \ar[rr] & & A \ar[d]^{=} \ar[rr] & & G \ar[d] \ar[rr] & & F \ar[d]^{=} \ar[rr] & & 0 \\
0 \ar[rr] & & A \ar[rr]& & G' \ar[rr] & & F \ar[rr] & & 0 \\
}
\]
One invariant of such a group extension is the conjugation action of $F$ on $A$: $G$ acts on $A$ via conjugation, and since $A$ acts on itself trivially, this action descends to an $F$-action on $A$. So let us fix an $F$-action on $A$ and try to classify all extensions giving rise to this fixed $F$-action on $A$. \\
Given an extension $0 \rightarrow A \rightarrow G \rightarrow F \rightarrow 0$, pick a set-theoretic section $s: F \rightarrow G$ with $s(1) = 1$. Usually, it will not be possible to choose $s$ as a group homomorphism; but at least $s(fg)$ and $s(f)s(g)$ project to the same element of $F$, namely $fg$, and hence only differ by an element $\phi(f,g)$ of $A$:
\[
s(f)s(g) = \phi(f,g)s(fg)
\]
Since $s(1) = 1$, it follows that $\phi(g,1) = 0 = \phi(1,f)$ for all $f,g \in F$. \\
Using $s$ and the inclusion $i: A \rightarrow G$, we can identify $G$ as a \emph{set} with $A \times F$ via $(a,f) \rightarrow i(a)s(f)$. To compute how to multiply two such elements, note that
\[
s(f)i(a) = i(fa)s(f)
\]
by definition of the conjugation action. So we compute
\begin{align*}
(a,f) \cdot (b,g) &= i(a)s(f)i(b)s(g)\\
 &= i(a)i(fb)s(f)s(g) \\
&= i(a+fb)s(f)s(g)\\
&= i(a+fb)\phi(f,g)s(fg) \\
&= (a+fb+\phi(f,g),fg)
\end{align*}
So we have completely recovered the extension we started with in terms of $\phi$ and the $F$-action on $A$. Note that if $s$ was a group homomorphism, $\phi = 0$ and we have recovered the semidirect product of $F$ and $A$. The section $s$ is also encoded into this picture: It is just the map $F\rightarrow A \times F, f \mapsto (f,0)$. Conversely, given $\phi: G \times G \rightarrow A$, we could try to define a group structure on $A \times F$ using the above formula. This will in general fail since the arising multiplication is not necessarily associative. Given $(a,f),(b,g), (c,h)$ and $\phi: G \times G \rightarrow A$, we compute
\[
((a,f)\cdot (b,g))\cdot(c,h) = (a+fb+\phi(f,g),fg)\cdot (c,h) = (a+fb+\phi(f,g)+fgc+\phi(fg,h), fgh)
\]
and
\[
(a,f)\cdot((b,g)\cdot (c,h)) = (a,f)\cdot(b+gc+\phi(g,h),gh) = (a+fb+fgc+f\phi(g,h)+\phi(f,gh), fgh)
\]
These two expressions are equal for all $f,g,h$ if and only if we have
\[
\phi(f,g)+\phi(fg,h) = f\phi(g,h)+\phi(f,gh)
\]
for all $f,g,h$. If this is true, the defined multiplication is associative and one easily verifies using $\phi(g,1) = 0 = \phi(1,f)$ that $(0,1)$ is an identity element and
\[
(a,f) \cdot (-f^{-1}a -f^{-1}\phi(f,f^{-1}), f^{-1}) = (0,1) 
\]
and hence $A \times G$ with this multiplication is a group. \\
Now what does this have to do with group cohomology? We may view $\phi: G \times G \rightarrow A$ as a $2$-chain of $\Hom(F,A)$

\fxnote{Change notation away from F}

\pagebreak

\section{The Witt ring functor for algebraic $K$-theorists}

This is an account of some of the theory of (big) Witt vectors. We will not consider $p$-adic Witt vectors, which are prominent in algebraic geometry, though the Burnside ring description of the Witt vector ring we will give can be generalised to cover this  case as well, see \cite{Dress-Witt} and \cite{elliott}. We refer the reader interested in $p$-adic Witt vectors to \cite{rabinoff}. However, the universal polynomial-type arguments given there can be quite confusing, and are not well-suited for the applications to algebraic $K$-theory. The approach presented here is more in the spirit of linear algebra, motivated by the amazing result of Almkvist in \cite{alm-endo} which we will review in \ref{almkvist} and the approach to Witt vectors presented in \cite{dayton}. Also the article of Hazewinkel \cite{Haze} on Witt vectors contains an amazing amount of information, though not many detailed proofs. Our coverage of the relationship between symmetric polynomials and Witt vectors is based on \cite{Haze}.

\subsection{The definition}

Let $R$ be a commutative ring and let $f: R^{n} \rightarrow R^{n}$ be a linear map. The basic observation underlying the ring of Witt vectors is the exponential trace formula, which relates the characteristic polynomial of $f$ to the traces of powers of $f$:

\begin{prop}
Let $\lambda_{f} = \det(1-tf)$ be the characteristic polynomial of $f$. Then we have in the ring $R[[t]]$ of formal power series over $R$ the identity
\[
-t \frac{d}{dt} \log(\lambda_{f}) = \sum\limits_{i=1}^{\infty} \trace(f^{i})t^{i}
\]
which we call the \emph{exponential trace formula}.
\end{prop}

\begin{rem}
The definition of the characteristic polynomial made here is not the usual linear algebra definition, but the information transported is nearly the same. If $\lambda(f) = 1+a_{1}t+a_{2}t^{2}+\cdots+a_{k}t^{k}$ and $f$ is an endomorphism of $R^{n}$, then the usual characteristic polynomial of $f$, namely $\det(t-f)$, is obtained by reversing the coefficients: it is
\[
t^{n}+a_{1}t^{n-1}+ \cdots + a_{k}t^{n-k}
\]
Hence the only information lost in $\lambda(f)$ compared to $\det(t-f)$ is the dimension of the $R$-module on which $f$ acts. For example, each zero endomorphism has characteristic polynomial $1$, independent of its size. 
\end{rem}

\begin{proof}
First assume that $R$ is an algebraically closed field. Then we may write $\lambda_{f} = \prod\limits_{i=1}^{n} (1-x_{i}t)$, where the $x_{i}$ are the eigenvalues of $f$ counted with multiplicity.  
Then we compute
\begin{align*}
-t \frac{d}{dt} \log(\prod\limits_{i=1}^{n} (1-x_{i}t)) &= \sum\limits_{i=1}^{n} \frac{x_{i}t \frac{\lambda_{f}}{1-x_{i}t}}{\lambda_{f}} \\  
&= \sum\limits_{i=1}^{n} \frac{x_{i}t}{1-x_{i}t} \\ 
&= \sum\limits_{i=1}^{n} (x_{i}t)(1+x_{i}t+x_{i}^{2}t^{2}+...) \\
&= \sum\limits_{i=1}^{n} \sum\limits_{k=1}^{\infty} x_{i}^{k}t^{k} \\
&= \sum\limits_{k=1}^{\infty} (\sum\limits_{i=1}^{n} x_{i}^{k})t^{k} \\
&= \sum\limits_{k=1}^{\infty} \trace(f^{k})t^{k}
\end{align*}
This also proves the formula for all subrings of algebraically closed fields. Now if $R$ is any ring, we find a ring surjection $p: A \rightarrow R$ with $A$ a subring of an algebraically closed field, for example $A = \IZ[\{ x_{r}\}_{r \in R}]$. Then $f: R^{n} \rightarrow R^{n}$ lifts to some map $g: A^{n} \rightarrow A^{n}$ and the formula holds for $g$. Applying $p$ to the formula for $g$, we obtain the formula for $f$.
\end{proof}

At this point, let us make the following definition:

\begin{definition}
A sequence $a_{i}$ in $R$ is a trace sequence if there is some $f: R^{n} \rightarrow R^{n}$ with $a_{i} = \trace(f^{i})$. Then we will call $a_{i}$ the trace sequence of $f$.
\end{definition}

Note that not all sequences are trace sequences. For example, over the integers, any sequence starting with $1, 0,...$ cannot be a trace sequence. To see this, note that we may also write the exponential trace formula as
\[
-t \lambda_{f}' = \lambda_{f} \cdot \sum\limits_{k=1}^{\infty}  \trace(f^{k})t^{k}
\]
Writing $\lambda_{f} = 1+b_{1}t+b_{2}t^{2}+...$ and comparing coefficients on both sides, we obtain a formula relating the $b_{i}$ to the trace sequence of $f$. The first two equations read
\begin{align*}
-b_{1} &=  \trace(f) \\
-2b_{2} &= \trace(f^{2}) + b_{1}\trace(f)
\end{align*}
Trying to solve these equations for $b_{1}$ and $b_{2}$ given $\trace(f) = 1$ and $\trace(f^{2}) = 0$ leads to $b_{1} = -1$ and $2b_{2} = -1$, which does not have an integral solution. And even if the recursion is solvable over the integers, it may happen that infinitely many of the coefficients $b_{i}$ are nonzero, yielding another reason why a sequence may not be a trace sequence. \\
In general, the recursive formulas relating the traces and the characteristic polynomial take the following form:

\begin{prop}
\label{recursion}
If $\lambda_{f}  = 1+a_{1}t+a_{2}t^{2}+...+a_{n}t^{n}$, the following identity holds for all $k > 0$:
\[
ka_{k}+\trace(f)a_{k-1}+\trace(f^{2})a_{k-2}+...+\trace(f^{k-1})a_{1}+\trace(f^{k}) = 0
\]
where we set $a_{k} = 0$ for $k > n$.
\end{prop}

\begin{proof}
Comparing coefficients in the formula $-t \lambda_{f}' = \lambda_{f} \cdot \sum\limits_{k=1}^{\infty}  \trace(f^{k})t^{k}$ yields the desired result.
\end{proof}
 
This formula also allows to reconstruct the characteristic polynomial of an endomorphism $f$ out of its trace sequence as long as the ring is of characteristic zero.  
 So in some sense, the traces are a kind of exotic or ghost coordinates for polynomials: Instead of remembering the coefficients of a polynomial $\lambda$, one may remember the coefficients of the formal power series $-t \frac{d}{dt} \log(\lambda)$ and then reconstruct the polynomial out of it. This may seem like a really stupid idea since $-t \frac{d}{dt} \log(\lambda)$ usually is an infinite power series, but some constructions are much more natural when expressed in these coordinates.

\begin{prop}
Let $f: R^{n} \rightarrow R^{n}$ and $g: R^{k} \rightarrow R^{k}$. Then the sequence obtained by pointwise multiplication of the trace sequences of $f$ and $g$ is a trace sequence.
\end{prop}

\begin{proof}
The product of the two trace sequences is the trace sequence of $f \otimes g$.
\end{proof}

So in our ghost coordinates, computing the characteristic polynomial of the tensor product of two endomorphisms out of the characteristic polynomials of the two endomorphisms is as easy as one might wish for: Just multiply the two sequences pointwise. Reading it off directly from the two known characteristic polynomials, however, is quite difficult. The idea of Witt vectors is to define a multiplication on the level of polynomials such that the transition from power series to our ghost coordinates is a ring homomorphism, where the operations on the ghost coordinates are pointwise. Then the Witt product of the two characteristic polynomials should be the characteristic polynomial of the tensor product of the original two endomorphisms. This cannot quite work as simply as that, mainly because polynomials usually do not have a multiplicative inverse. However, the ghost map makes perfect sense for any power series with leading coefficient $1$, so we may ask the following question:

\begin{problem}
Is there a ring structure on $1+tR[[t]]$such that the ghost map
\[
\gh = -t \frac{d}{dt} \log: 1+tR[[t]] \rightarrow  \prod\limits_{i=1}^{\infty} R
\]
is a ring homomorphism? Equivalently, is there a ring structure on $1+R[[t]]$ such that all the components $\gh_{n}$ of $\gh$ are ring homomorphisms $\gh_{n}: 1+R[[t]] \rightarrow R$? 
\end{problem}

Here, we identify a sequence $(a_{1},a_{2},...) \in \prod\limits_{i=1}^{\infty} R$ with the power series $\sum\limits_{i=1}^{\infty} a_{i}t^{i}$ and use the pointwise multiplication and addition on $\prod\limits_{i=1}^{\infty} R$. \\
What the addition on $1+tR[[t]]$ should be is easy to see. Indeed, if $f: R^{n} \rightarrow R^{n}$ and $g: R^{k} \rightarrow R^{k}$ are linear, the sum of the trace sequences of $f$ and $g$ is the trace sequence of $f \oplus g$, and the characteristic polynomial of $f \oplus g$ is the \emph{product} of the characteristic polynomials of $f$ and $g$. So addition on $1+tR[[t]]$ should be the ordinary multiplication of power series. This indeed works out:

\begin{prop}
The ghost map
\[
-t \frac{d}{dt} \log: 1+tR[[t]] \rightarrow  \prod\limits_{i=1}^{\infty} R
\]
is a group homomorphism, where the left-hand side is a group under the multiplication of power series.
\end{prop}

\begin{proof}
We compute for any two power series $f,g$
\begin{align*}
-t \frac{d}{dt} \log(fg) &= -t \frac{d}{dt} (\log(f)+\log(g)) \\
&= -t \frac{d}{dt} \log(f) +  (-t \frac{d}{dt} \log(g))
\end{align*}
which is what we wanted to prove.
\end{proof}
 
Multiplication is more subtle. Let us begin with the following fact:

\begin{prop}
\label{recursive}
If $R$ is a field of characteristic $0$, the ghost map $-t \frac{d}{dt} \log$ is a bijection. Consequently, there is a unique ring structure on $1+tR[[t]]$ making the ghost map a ring isomorphism. If $R$ is of characteristic $0$, the ghost map is injective.
\end{prop}

\begin{proof}
The proof of \ref{recursion} also applies to power series, so we have for a power series $f = 1+a_{1}t+a_{2}t^{2}+...$ the identites
\[
ka_{k}+\gh_{1}(f)a_{k-1}+\gh_{2}(f)a_{k-2}+...+\gh_{k-1}(f)a_{1}+\gh_{k}(f) = 0
\]
Over a field of characteristic $0$, no matter what sequence $\gh(f)$ is, we can solve for the $a_{i}$ since we can divide by any natural number $k$. If $R$ is not a field, but at least of characteristic $0$, multiplication by $k$ is injective on $R$, so while not any sequence is in the image of the ghost map (it is if and only if the recursions are solvable over $R$), at least there is at most one solution. This proves the claim.
\end{proof}

So for a field of characteristic $0$, we have solved our problem, and we at least know that there is at most one possible multiplication on a ring of characteristic $0$. However, for an arbitrary ring, the Witt multiplication (whose existence is still wishful thinking) may not be uniquely defined, since the ghost map may not be injective. But there is one further property we would like to force on our multiplication which will imply uniqueness of the Witt multiplication. \\ \\
Let us return to our linear algebra example. Let $f: R^{n} \rightarrow R^{n}$ and $g: R^{k} \rightarrow R^{k}$ be linear endomorphisms and $\phi: R \rightarrow S$ a ring homomorphism. We get induced maps $\phi(f): S^{n} \rightarrow S^{n}$ and $\phi(g): S^{k} \rightarrow S^{k}$. We also have $\phi(f \otimes g) = \phi(f) \otimes \phi(g)$, so the characteristic polynomial of $\phi(f) \otimes \phi(g)$ may be computed by pushing forward the characteristic polynomial of $f \otimes g$ via $\phi$. \\
On the other hand, we should also be able to compute the characteristic polynomial of $\phi(f) \otimes \phi(g)$ as the Witt product of the characteristic polynomials of $\phi(f)$ and $\phi(g)$. In other words, our Witt multiplication should be natural with respect to $\phi$: we get an induced map $\phi[[t]]: 1+tR[[t]] \rightarrow 1+tR[[t]]$ by applying $\phi$ to the coefficients, and by the above considerations, it is natural to demand that this map is a ring homomorphism.  In other words, we would like that sending $R$ to $1+tR[[t]]$ with our desired ring structures is a functor from rings to rings. Then we immediately obtain uniqueness of our potential multiplication:

\begin{prop}
There is at most one functor $W: Crings \rightarrow Crings$ with the following properties:
\begin{enumerate}
\item On the set level, $W$ is given by $R \mapsto 1+tR[[t]]$ and a ring homomorphism $\phi: R \rightarrow S$ is sent to $W(\phi): 1+tR[[t]] \rightarrow 1+tS[[t]]$ which is given by applying $\phi$ to the coefficients of the power series.
\item The ghost map $-t \frac{d}{dt}\log: 1+tR[[t]] \rightarrow \prod\limits_{i=1}^{\infty}$ is a ring homomorphism.
\end{enumerate}
\end{prop}

\begin{proof}
We already saw that condition (ii) forces uniqueness of the ring structure as long as $R$ is of characteristic $0$. If $R$ is an arbitrary ring, we find a ring surjection $\phi: A \rightarrow R$ with $A$ of characteristic $0$. Given $f,g$ in $1+tR[[t]]$, we find $p,q \in 1+tA[[t]]$ with $\phi[[t]](p) = f$, $\phi[[t]](q) = g$ since $\phi$ is surjective. Now condition (i) forces that the product of $f$ and $g$ is $\phi[[t]]$ applied to the product of $p$ and $q$, which we already know is unique. Hence the product of $f$ and $g$ is unique. The same argument applies to addition.
\end{proof}

Now we can turn to the question of existence of our desired multiplication. This is a bit more complicated; we first deal with the case of characteristic $0$-rings. 

\begin{prop}
Let $M$ be the category of rings of characteristic $0$. Then there is a functor $W: M \rightarrow Crings$ with the two properties formulated above.
\end{prop}

\begin{proof}
For rings of characteristic $0$, the ghost map $-t \frac{d}{dt}\log: 1+tR[[t]] \rightarrow \prod\limits_{i=1}^{\infty} R$ is injective. We hence only have to see that the image  is a subring of $\prod\limits_{i=1}^{\infty} R$; then we can pull back the ring structure of this subring to $1+tR[[t]]$. Since we already dealt with addition, we only have to consider multiplication. \\  
First note that $1,1,1,...$ is a trace sequence, namely the trace sequence of the identity of $R$. So the $1$ of $\prod\limits_{i=1}^{\infty} R$ is in the image of the ghost map. Now, if $p, q \in 1+R[[t]]$ are actual polynomials, we may find endomorphisms $f, g$ of free $R$-modules such that $p = \lambda_{f}$ and $q = \lambda_{g}$. Then the product of the trace sequences of $f$ and $g$ is the trace sequence of $f \otimes g$, hence the product of the ghost sequences of $p$ and $q$ are again in the image of the ghost map. \\
We can now use a continuity argument to extend this to arbitrary $p$ and $q$. Inspecting \ref{recursive}, one finds that $\gh_{n}(p)$ only depends on the first $n$ coefficients of $p$. In other words, putting the $t$-adic topology on $1+R[[t]]$ and the product topology on $\prod\limits_{i=1}^{\infty} R$, the ghost map is continuous. This also works the other way around: When retrieving the coefficients of $p$ out of $\gh(p)$, one finds that the $n$-th coefficient of $p$ only depends on the $\gh_{i}(p)$ with $i  \leq n$. It follows that the image of $\gh$ is closed. Approximating $p$ and $q$ by sequences $p_{i}$ and $q_{i}$ of polynomials, $\gh(p) \cdot \gh(q)$ is the limit of $\gh(p_{i}) \cdot \gh(q_{i})$ which is in the image of the ghost map. Hence 
$\gh(p) \cdot \gh(q)$ is in the image of the ghost map, proving the claim. \\
To extend this to arbitrary rings, we will employ what one might call a Yoneda trick. The underlying set of $W(R)$ defines a functor from the category of rings of characteristic $0$ to sets, and this functor is represented by the ring $\IZ[\{ x_{i}\}_{i \in \IN}]$, i.e. we have a natural isomorphism of sets
\[
W(R) \cong \Hom_{Rings}(\IZ[\{ x_{i}\}_{i \in \IN}] ,R)
\]
Indeed, both sides can be identified with an infinite countable product of copies of $R$. Now we have already lifted $W(-)$ to a functor to commutative rings. By the Yoneda lemma, another way to view this is that we have already defined additional structure on $\IZ[\{ x_{i}\}_{i \in \IN}]$. For example, the product of $W(R)$ gives rise to a map
\[
\Hom_{Rings}(\IZ[\{ x_{i}\}_{i \in \IN}] ,R) \times \Hom_{Rings}(\IZ[\{ x_{i}\}_{i \in \IN}] ,R) \rightarrow \Hom_{Rings}(\IZ[\{ x_{i}\}_{i \in \IN}] ,R)
\]
which is natural in $R$, i.e. a natural transformation of functors
\begin{align*}
\Hom_{Rings}(\IZ[\{ x_{i}\}_{i \in \IN}]  \otimes_{\IZ} \IZ[\{ x_{i}\}_{i \in \IN}] ,-) \cong \\ \Hom_{Rings}(\IZ[\{ x_{i}\}_{i \in \IN}] ,-) \times \Hom_{Rings}(\IZ[\{ x_{i}\}_{i \in \IN}] ,-) \\ \cong \Hom_{Rings}(\IZ[\{ x_{i}\}_{i \in \IN}] ,-)
\end{align*}
which, by the Yoneda lemma, has to be given by a map of rings
\[
\IZ[\{ x_{i}\}_{i \in \IN}] \rightarrow \IZ[\{ x_{i}\}_{i \in \IN}]  \otimes_{\IZ} \IZ[\{ x_{i}\}_{i \in \IN}] 
\]
Note that we can indeed employ the Yoneda lemma because $\IZ[\{ x_{i}\}_{i \in \IN}]  \otimes_{\IZ} \IZ[\{ x_{i}\}_{i \in \IN}] $ is of characteristic $0$ and hence a ring for which the functor $W$ was already defined.
Associativity and commutativity of the multiplication on $W(R)$ can be encoded as properties of this map. In the end, $\IZ[\{ x_{i}\}_{i \in \IN}]$ is something like a coalgebra object in commutative rings. Now we can plug in an arbitrary ring $R$ and get a map 
  \[
\Hom_{Rings}(\IZ[\{ x_{i}\}_{i \in \IN}] ,R) \times \Hom_{Rings}(\IZ[\{ x_{i}\}_{i \in \IN}] ,R) \rightarrow \Hom_{Rings}(\IZ[\{ x_{i}\}_{i \in \IN}] ,R)
\]
which is the multiplication on $W(R)$. The same argument applies to all other structures.
\end{proof}

There is another description of the ghost coordinate map, coming from the fact that there are several different ways of identifying the set $1+tR[[t]]$ with the infinite product $\prod\limits_{i=1}^{\infty} R$. We just used the obvious one, identifying the power series $1+a_{1}t+a_{2}t^{2}+...$ with the sequence $a_{1}, a_{2}, ...$. But there is another possibility commonly used in connection with the Witt ring functor:

\begin{prop}
Each power series in $1+tR[[t]]$ has a unique decomposition as an infinite product of the form $\prod\limits_{i=1}^{\infty} (1-b_{i}t^{i})$.
\end{prop}

\begin{proof}
Since $1+tR[[t]]$ is a group under multiplication, it suffices to see that the inverse of any power series $p = 1+a_{1}t+a_{2}t^{2}$ may be written in the form $\prod\limits_{i=1}^{\infty} (1-b_{i}t^{i})$. We start by setting $b_{1} = a_{1}$. Then we have $p(1-b_{1}t) = 1+c_{2}t^{2}+c_{3}t^{3}$  with some coefficients $c_{i} \in R$ and set $b_{2} = c_{2}$. Now, $p(1-b_{1}t)(1-b_{2}t^{2}) = 1+d_{3}t^{3}+d_{4}t^{4}+...$ and we set $b_{3} = d_{3}$. Proceeding in this way, we obtain a sequence $b_{i}$ such that  $\prod\limits_{i=1}^{\infty} (1-b_{i}t^{i})$ is the inverse of $p$, proving the claim.
\end{proof}

\begin{prop}
Identifying a sequence $a_{i}$ with the power series $\prod\limits_{i=1}^{\infty} (1-a_{i}t^{i})$, the ghost coordinate map takes the form
\[
\gh_{n}((a_{i})_{i \in \IN}) = \sum\limits_{d \mid n} d a_{d}^{\frac{n}{d}}
\]
\end{prop}

\begin{proof}
We compute
\begin{align*}
-t \frac{d}{dt} \log \prod\limits_{i=1}^{\infty} (1-b_{i}t^{i}) &= -t \frac{d}{dt} \sum\limits_{i=1}^{\infty} \log(1-a_{i}t^{i}) \\
&= -t \sum\limits_{i=1}^{\infty} \frac{-ia_{i}t^{i}}{1-a_{i}t^{i}} \\
&= \sum\limits_{i=1}^{\infty} ia_{i}t^{i}(1+a_{i}t^{i}+a_{i}^{2}t^{2i}+...)
\end{align*}
The coefficient of $t^{n}$ in the last sum is easily checked to be the desired expression.
\end{proof}

Often, these formulaes are taken as the (largely unmotivated) starting point for the definition of Witt vectors; in the approach presented here, these formulaes just show up naturally.

\subsubsection{Frobenius and Verschiebung}

There are two important families of operations on the Witt ring: The Frobenius maps and the Verschiebung maps. For each natural number $n$, these are natural group homomorphisms $F_{n}, V_{n}: W(R) \rightarrow W(R)$. Their defininig property is their relationship with the ghost coordinates:  We have
\[
\gh_{k}(F_{n}(x)) = \gh_{kn}(x)
\]
and
\[
\gh_{k}(V_{n}(x)) = \begin{cases} 
0 &\text{ if } n \nmid k \\
n \cdot \gh_{\frac{k}{n}} &\text{ if } n \mid k
\end{cases}
\]
Indeed, if $R$ is a field of characteristic $0$, this already defines $F_{n}$ and $V_{n}$ since $\gh: W(R) \rightarrow \prod R$ is an isomorphism, so we can pull back any map defined only on ghost coordinates to a map of the Witt ring. Since both $\gh_{k} \circ F_{n}$ and $\gh_{k} \circ V_{n}$ are group homomorphisms for all $n$ and $k$, it follows that $V_{n}: W(R) \rightarrow W(R)$ and $F_{n}: W(R) \rightarrow W(R)$ are group homomorphisms. Furthermore, $\gh_{k} \circ F_{n}$ is even a ring homomorphism, so $F_{n}$ also is   a ring homomorphism. \\
To extend these constructions to an arbitary ring $R$, we will again employ the Yoneda trick used above: Once we have $F_{n}$ and $V_{n}$ for all rings of characteristic $0$, we can view them as additional structures on the ring $\IZ[\{x_{i}\}]$ representing the Witt ring functor, and then the oeprations can be extended to all rings. So assume that $R$ is of characteristic zero. Since the ghost map is injective in this case, we only have to see that for any $x \in \prod R$ which is in the image of the ghost map, the sequences $y_{i}$ and $z_{i}$ defined by
\[
y_{k} = x_{kn}
\]
and
\[
z_{k} = \begin{cases} 
0 &\text{ if } n \nmid k \\
n \cdot x_{\frac{k}{n}} &\text{ if } n \mid k
\end{cases}
\]
are also in the image of the ghost map. If $x$ is actually a trace sequence, i.e. there is some endomorphism $f: R^{m}\rightarrow R^{m}$ such that $\tr(f^{i}) = x_{i}$, then it is immediate that the sequence $y_{k}$ is the trace sequence of $f^{n}$. Let $V(f): R^{nm} \rightarrow R^{nm}$ be given by the matrix of $m \times m$-matrices
\[
 \begin{pmatrix}
0 & 0 & 0 & .... & f \\
\Id_{R^{m}} & 0 & 0 & ... & 0 \\
0 & Id_{R^{m}} & 0 & ... & 0 \\
... & ... & ... & ... & ... & \\
0 & 0 & ... & Id_{R^{m}} & 0 \\

\end{pmatrix})
\]
A computation shows that $z_{i} = \tr(V(f)^{i})$. If $x$ is arbitrary, we can approximate $x$ by trace sequences $x^{j}$; the sequences $y^{j}$ and $z^{j}$ we have just defined will then approximate $y$ and $z$. Since all $y^{j}$ and $z^{j}$ are trace sequences, their limits also have to be in the image of the ghost map, and this is what we wanted to see.

\fxnote{put somewhere the proposition ghost sequence iff each cutoff sequence is part of a trace sequence?}

Alltogether, we obtain the following:

\begin{prop}
There are group endomorphisms $F_{n}, V_{n}: W(R) \rightarrow W(R)$, natural in the ring $R$. Furthermore, $F_{n}$ is even a ring homomorphism.
\end{prop}

The basic properties of the Frobenius and Verschiebung are subsumed in the following proposition:

\begin{prop}
The $F_{n}$ and $V_{n}$ satisfy the following additional relations:
\begin{enumerate}
\item $F_{n} \circ V_{n}$ is multiplication with $n$.
\item $F_{m} \circ F_{n} = F_{mn}$
\item On the level of power series, $V_{n}$ is given by $p(t) \rightarrow p(t^{n})$. Correspondingly, we have $V_{m} \circ V_{n} = V_{mn}$
\item $V_{m} \circ F_{n} = F_{n} \circ V_{m}$ if $gcd(m,n) = 1$.
\item $F_{m}$ is a ring homomorphism.
\item $V_{m}(a * F_{m}(b)) = (V_{m}(a)) * b$ where $*$ is the multiplication in $\bend_{0}(R)$.
\end{enumerate}
\end{prop}

\begin{proof}
This is really a statement about the operations on the representing ring of the Witt ring functor, so we can restrict to rings of characteristic $0$. For such rings, two elements of the Witt ring are equal if and only if all their ghost coordinates agree. It is now a lengthy, but easy calculation to prove all the relationships we have listed. For example, we find that
\[
\gh_{k}(F_{n}(V_{n}(x)) = \gh_{kn}{V_{n}(x)} = n \cdot \gh_{k}(x)
\]
Since also $\gh_{k}(nx) = n\gh_{k}(x)$, we must have $nx = F_{n}(V_{n}(x)$. All other claims are proved in the same way. 
\end{proof}

This behaviour can also be explained by linear algebra, and actually we have already seen which operations in linear algebra correspond to the Frobenius and Verschiebung maps: The Frobenius encodes passing from an endomorphism $f$ of some $R^{m}$ to $f^{n}$, whereas the Verschiebung corresponds to the endomorphism $V(f)$ defined above. 

\subsection{Even closer ties to linear algebra}

So far, we have used linear algebra over the commutative ring $R$ mainly as a motivational source. However, it turns out that we can describe the Witt ring directly through linear algebra. For this, we make the following definition. \fxnote{backreference to the part in the main text where we define this}

\begin{definition}
The \emph{endomorphism category} $\bend(P(R))$ of $R$ is the category with objects pairs $(P,f)$ with $P$ an object of $P(R)$ and $f: P \rightarrow P$ an endomorphism of $P$. A morphism from $(P,f)$ to $(Q,g)$ in $\bend(R)$ is a morphism $\phi: P \rightarrow Q$ in $P(R)$ such that $\phi \circ f = g \circ \phi$. The category $\bend(P(R))$ inherits an exact structure from $P(R)$ by declaring a sequence in $\bend(P(R))$ to be exact if and only if its underlying sequence in $P(R)$ is exact. Analogously, we define $\bend(H(R))$.
\end{definition}
 Note that the exact structure on $\bend(P(R))$ is not split, even though the exact structure on $P(R)$ is. We are interested in $K_{0}(\bend(P(R)))$. An easy resolution argument shows  $K_{0}(\bend(P(R))) = K_{0}(\bend(H(R)))$. Furthermore, there is an exact functor $P(R) \rightarrow \bend(P(R))$ sending $P$ to $(P,0)$ which splits the projection functor $\bend(P(R)) \rightarrow P(R)$. Hence there is a splitting
\[
K_{0}(\bend(P(R))) = K_{0}(R) \oplus \bend_{0}(R)
\]
Here, $\bend_{0}(R)$ is the Grothendieck group of $\bend(P(R))$ with the additional relation that $(P,0) = 0$ for all $P$. This  group is computed in \cite{Alm}.

First note that for $\bend_{0}(R)$, we may as well assume that all involved modules are free: If $(P,f)$ is any object in $\bend(R)$, there is a complement $Q$ to $P$ with $Q \oplus P$ free and hence a short exact sequence

\[
\xymatrix{
0 \ar[rr] & & P \ar[d]^{f} \ar[rr] & & P \oplus Q \ar[d]^{f \oplus 0} \ar[rr] & & Q \ar[d]^{0} \ar[rr] & & 0 \\
0 \ar[rr] & & P \ar[rr] & & P \oplus Q  \ar[rr] & & Q  \ar[rr] & & 0
}
\]

which means $(P,f) = (P \oplus Q, f \oplus 0) - (Q,0)$ in $K_{0}(\bend(P(A)))$ and hence $(P,f) = (P \oplus Q, f \oplus 0)$ in $\bend_{0}(A)$. Let $Q(R)$ be the group of all rational functions in $R$ of the form
\[
\frac{1+a_{1}t+...+a_{n}t^{n}}{1+b_{1}t+...+b_{n}t^{n}}
\]
i.e. with both nominator and denominator having constant term $1$. The group operation is multiplication. We define a map $\lambda: \bend_{0}(A) \rightarrow Q(R)$ by sending $(R^{n},f)$ to $\chi(t) = \det(1-tf)$. This is indeed well-defined since the characteristic polynomial is additive with respect to short exact sequences. We can now state Almkvist's theorem:

\begin{thm}
\label{almkvist}
The map $\lambda$ is an isomorphism of groups.
\end{thm}

\begin{proof}
See \cite{alm-endo}.
\end{proof}

The group $\bend_{0}(A)$ is also a ring under the tensor product, and $Q(R)$ is actually a subring of the Witt ring. The isomorphism $\lambda$ respects this ring structure:

\begin{prop}
The map $\lambda$ is an isomorphism of rings.
\end{prop}

\begin{proof}
We already now that $\lambda$ is an isomorphism, and it is clearly natural with respect to ring homomorphisms. Since an injection of rings $R \rightarrow S$ induces a ring injection $Q(R) \rightarrow Q(S)$ and correspondingly a ring injection $\bend_{0}(R) \rightarrow \bend_{0}(S)$, $\lambda$ is a ring homomorphism for $R$ if it is a ring homomorphism for $S$. A similar statement holds for surjections of rings. Since any ring is a quotient of a subring of an algebraically closed field, it is enough to check the claim for an algebraically closed field $F$. Let $f: F^{n} \rightarrow F^{n}$ and $g: F^{m} \rightarrow F^{m}$ be endomorphisms with characteristic polynomials $\chi(f) = \prod\limits_{i=1}^{n}(1-\lambda_{i}t)$ and $\chi(g) = \prod\limits_{i=1}^{m}(1-\mu_{i}t)$. Then the characteristic polynomial of their tensor product is $\prod\limits_{i,j} (1-\lambda_{i} \mu_{j}t)$, which is easy to check since the tensor product of two upper triangular matrices is upper triangular. But the multiplication in the Witt ring is designed such that $(1-at)(1-bt) = 1-abt$, and the claim follows.
\end{proof}

Now we turn to the definition of the Frobenius and Verschiebung in this picture of the Witt ring functor. For each $n \in \IN$, there are exact functors $F_{n}, V_{n}: \bend(P(R)) \rightarrow \bend(P(R))$ given by

\[
F_{n}(P,f) = (P, f^{n})
\]

respectively

\[
V_{n}(P,f) = (P^{n}, \begin{pmatrix}
0 & 0 & 0 & .... & f \\
Id_{P} & 0 & 0 & ... & 0 \\
0 & Id_{P} & 0 & ... & 0 \\
... & ... & ... & ... & ... & \\
0 & 0 & ... & Id_{P} & 0 \\

\end{pmatrix})
\]
These functors induce homomorphisms $\End_{0}(R) \rightarrow \End_{0}(R)$ which will be denoted by $V_{n}$ and $F_{n}$ again.

\begin{definition}
The $F_{n}$ are called the \emph{Frobenius maps} and the $V_{n}$ the \emph{Verschiebung maps} on $\bend_{0}(R)$.
\end{definition}

This terminology is of course motivated by the terminology in the Witt Ring; we will later see that under the identification of $\bend_{0}(R) \cong Q(R) \subset W(R)$, the Witt ring operations and the operations just defined agree. 

\begin{prop}
The $F_{n}$ and $V_{n}$ are group homomorphisms satisfying the following additional relations:
\begin{enumerate}
\item $F_{n} \circ V_{n}$ is multiplication with $n$.
\item $F_{m} \circ F_{n} = F_{mn}$
\item On the level of the characteristic polynomial, $V_{n}$ is given by $p(t) \rightarrow p(t^{n})$. Correspondingly, we have $V_{m} \circ V_{n} = V_{mn}$
\item $V_{m} \circ F_{n} = F_{n} \circ V_{m}$ if $gcd(m,n) = 1$.
\item $F_{m}$ is a ring homomorphism.
\item $V_{m}(a * F_{m}(b)) = (V_{m}(a)) * b$ where $*$ is the multiplication in $\bend_{0}(R)$.
\end{enumerate}
\end{prop}

\begin{proof}
For (i), note that already on the exact functor level, $V_{n}(F_{n}(P,f)) = (P^{n}, f^{\oplus n})$. The claim then easily follows. Item (ii) is already true on the exact functor level. \\
The other four identities are proven by reduction to the universal case. For instance, the claim in (vi) says that the two bilinear maps
\[
V_{m}(- * F_{m}(-)), V_{m}(-) * (-): \bend_{0}(R) \times \bend_{0}(R) \rightarrow \bend_{0}(R)
\]
are equal. If the claim is true for a ring $R$, it is true for any subring $S$ of $R$ since the induced map $\bend_{0}(S) \rightarrow \bend_{0}(R)$ is injective and both maps under consideration are natural with respect to ring homomorphisms. Similarly, if $f: R \rightarrow S$ is a surjective ring homomorphism and the claim is true for $R$, it follows for $S$ because  $\bend_{0}(R) \rightarrow \bend_{0}(S)$ is surjective as well. So we can reduce to the case of an algebraically closed field $F$ and to the case where $a$ is multiplication by $\lambda$ on $F$ and $b$ is multiplication by $\mu$ on $F$. Since $\bend_{0}(R) \cong Q(R)$ via the characteristic polynomial, it is sufficient to verify the relation on characteristic polynomials. There we have
\[
V_{m}((1-\lambda t) * F_{m}(1-\mu t)) = V_{m}((1-\lambda t)*(1-\mu^{m} t) = V_{m}(1-\mu^{m} \lambda t) = 1-\mu^{m} \lambda t^{m}
\]
and
\[
V_{m}(1-\lambda t) * (1-\mu t) = (1-\lambda t^{m}) * (1-\mu t) = 1-\mu^{m} \lambda t^{m}
\]
and the claim follows. In the same way, one reduces (iii)-(v) to the case of an algebraically closed field. Item (iii) then directly follows from the computation in characteristic polynomials
\[
V_{n}(\prod\limits_{i=1}^{n} (1-a_{i} t)) = \prod\limits_{i=1}^{n} V_{n}(1-a_{i} t) = \prod\limits_{i=1}^{n} (1-a_{i} t^{n})
\]
Item (v) follows from a similar computation. For (iv), we compute
\[
F_{m} V_{n} (1-at) ) = F_{m} (1-at^{n}) = F_{m} (\prod\limits_{i=1}^{n} (1-b \chi^{i} t)) = \prod\limits_{i=1}^{n} (1-b^{m}\chi^{im} t) 
\]
where $b$ is an $n$-th root of $a$ and $\chi$ is a primitive $n$-th root of unity, and
\[
V_{n} F_{m} (1-at) = V_{n} (1-a^{m}t) = 1-a^{m}t^{n} 
\]
But thanks to the fact that $gcd(m,n)=1$, $\chi^{im}$ still runs through all $n$-th roots of unity, hence the first polynomial has precisely the $n$-th roots of $a^{-m}$ as zeros. This implies that the two polynomials are actually equal.
\end{proof}

There is also an easy way to describe the ghost components of the Witt ring in terms of $\bend_{0}(R)$:

\begin{definition}
Let $\gh_{n}: \bend_{0}(R) \rightarrow R$ be the group homomorphism given by $\gh_{n}(P,f) = \trace(f^{n})$.
\end{definition}

It is easy to check that this is well-defined. We have the following facts:

\begin{prop}
The maps $\gh_{n}$ are ring homomorphisms. Furthermore, we have 
\[
\gh_{n} \circ F_{m} = \gh_{nm}
\]
and
\[
\gh_{n}(V_{m}(x)) = \begin{cases} m \cdot \gh_{\frac{m}{n}}(x) & \text{if n divides m} \\ 0 & \text{else} \end{cases}
\]
\end{prop}

\begin{proof}
Since the trace of the tensor product of two endomorphisms is the product of the traces, $\gh_{n}$ is a ring homomorphism. The two identities are true on-the-nose, though this may not be quite obvious in the second case. However, an easy exercise in matrix multiplication will convince the reader that this is in fact true.
\end{proof}

We now identify the above constructions with the usual constructions on the Witt ring:

\begin{prop}
The Frobenius, Verschiebungs and ghost maps of $W(R)$ restrict to $Q(R)$ and are given by the $F_{n}, V_{n}$ and $\gh_{n}$ constructed above
\end{prop}

\begin{proof}
Consider the various Frobenius and Verschiebung maps as maps $Q(R) \rightarrow W(R)$. They are all group homomorphisms and natural with respect to ring homomorphisms. The usual argument allows us to restrict to the case of an algebraically closed field. There, both Verschiebung maps are given by $(1-at) \mapsto (1-at^{n})$ and both Frobenius maps are given by $(1-at) \mapsto (1-a^{n}t)$. A similar argument applies to the ghost maps. In particular, the Frobenius and Verschiebung maps indeed restrict to maps $Q(R) \rightarrow Q(R)$.
\end{proof}

\subsection{Symmetric functions and Witt rings}

Witt vectors are also closely related to the theory of symmetric functions. For example, if $p$ is a polynomial with constant coefficient $1$ over an algebraically closed field, we may write $p(t) = \prod\limits_{i=1}^{n} (1-x_{i}t)$. Writing out what the ghost coordinates and Frobenius are in terms of the $x_{i}$, we find

\begin{align*}
\gh_{k}(p) &= \sum\limits_{i=1}^{n} x_{i}^{k} \\
F_{k}(p) &= \prod\limits_{i=1}^{n} (1-x_{i}^{k}t)
\end{align*}

Both expressions are symmetric in the $x_{i}$ and hence can be expressed in the elementary symmetric functions in the $x_{i}$, i.e. the coefficients of $p$. Being courageous enough, one could try to \emph{define} the ghost coordinates and Frobenius in this way: Writing a polynomial $p$ over any ring formally as $p(t) = \prod\limits_{i=1}^{n} (1-x_{i}t)$, then forming 
$\sum\limits_{i=1}^{n} x_{i}^{k}$ respectively $\prod\limits_{i=1}^{n} (1-x_{i}^{k}t)$ and expressing these in terms of the elementary symmetric functions in the $x_{i}$, i.e. the coefficients of $p$.
For polynomials, this actually works; however, we are interested in power series and hence have to consider infinite products $\prod\limits_{i=1}^{\infty} (1-x_{i}t)$ and symmetric functions in infinitely many variables. 

\begin{definition}
Let $R$ be a ring, $x_{1}, x_{2}, \dots$ infinitely many commuting variables and $R[[x_{1}, x_{2},\dots]]$ the corresponding power series ring in infinitely many variables. Let $\Gamma(R)$ be the subring of $R[[x_{1}, x_{2},...]]$ which consists of the power series whose monomials have bounded degree. %terminal case of foot-in-mouth...
The ring $\Gamma(R)$ carries an action of the infinite symmetric group; let $\Lambda(R)$ be the fixed ring of this action, the \emph{ring of symmetric functions}. We write $h_{n}$  for the symmetric function $\sum\limits_{\#I = n} \prod\limits_{i \in I} x_{i}$. 
\end{definition}

The following is the analogue of the fundamental theorem of symmetric polynomials:

\begin{prop}
The ring $\Lambda(R)$ is the polynomial ring in the functions $h_{i}$.
\end{prop}

\begin{proof}
First we prove the algebraic independence of the $h_{i}$. Assume there is a polynomial $p$ over $R$ in $n$ variables such that $p(h_{1}, h_{2}, \dots h_{n}) = 0$. This is still true when setting $x_{i} = 0$ for all $i > n$, and then the algebraic independence of the first $n$ elementary symmetric polynomials in the $n$ variables $x_{1},\dots x_{n}$ forces $p = 0$. \\
Now let $S$ be any element of $\Lambda(R)$, with the degree of the monomials occuring in $S$ bounded by $n$. Again setting all variables $x_{i}$ with $i > n$ $0$, we obtain a symmetric polynomial $S_{n}$ in the finitely many variables $x_{1}, \dots x_{n}$. \fxnote{continue}
\end{proof}

Now we consider the ring $\Lambda(\IZ)[[t]]$. By the above result, $\Lambda(\IZ)$ is a polynomial ring in infinitely many variables, so $\Lambda(\IZ)[[t]]$ contains the universal power series $U = 1+h_{1}t+h_{2}t^{2}+...$: Given any power series $p$ over any ring $R$, there is a unique ring homomorphism $\phi: \Lambda(\IZ) \rightarrow R$ such that $\phi[[t]](U) = p$. However, we can also write $U$ as $\prod\limits_{i=1}^{\infty} (1-x_{i}t)$ and view this as a formal splitting of the power series $p$. For example, to define the Frobenius $F_{n}(p)$, we can consider the power series $F_{n}(U) = \prod\limits_{i=1}^{\infty} (1-x_{i}^{n}t)$. This power series is still symmetric, hence an element of $\Lambda(\IZ)$. Now define $F_{n}(p) = \phi[[t]](F_{n}(U))$. Similarly, the ghost coordinates are given on the universal power series by $\gh_{n}(U) = \sum_{i=1}^{\infty} x_{i}^{n}$. \fxnote{Proofs?}

\subsubsection{$\lambda$-rings}

Another construction which is hard to write down directly, but becomes quite natural in the symmetric functions point of view, is the $\lambda$-ring structure on the ring of Witt vectors. If $R$ is any commutative ring, we define exterior power operations $\lambda_{n}: W(R) \rightarrow W(R)$ as follows: On the universal power series $U$, we set
\[
\lambda_{n}(U) = \prod\limits_{i_{1} < i_{2} <  \dots < i_{n}} (1-x_{i_{1}}x_{i_{2}}\dots x_{i_{n}}t)
\]
If $p \in W(R)$ is any power series, we obtain a ring homomorphism $\phi: \Lambda(\IZ) \rightarrow R$ with $\phi[[t]](U) = p$ and set $\lambda_{n}(p) = \phi[[t]](\lambda_{n}(U))$. \fxnote{Why is this a good definition?}

\begin{prop}
The exterior power operations are natural with respect to ring homomorphisms $\phi: R \rightarrow S$: We have $\lambda_{n} \circ W(\phi) = W(\phi) \circ \lambda_{n}$.
\end{prop}

\begin{proof}
\fxnote{Add; is this obvious?}
\end{proof}

Of course, in a $\lambda$-ring, the exterior power operations have to satisfy certain equations. The easiest way to express this is as follows: 

\begin{definition}
Let $R$ be a ring together with maps $\lambda_{n}: R \rightarrow R$. The ring $R$ together with these operations is a pre-$\lambda$-ring if the map
\begin{align*}
\lambda: R &\rightarrow W(R) \\
x &\mapsto 1+\lambda_{1}(x)t+\lambda_{2}(x)t+\dots
\end{align*}
is a group homomorphism, i.e. if  $\lambda(x+y) = \lambda(x)\lambda(y)$. The ring $R$ is a $\lambda$-ring if $\lambda$ is a homomorphism of $\lambda$-rings, i.e. $\lambda$ is a ring homomorphism and we have $\lambda(\lambda_{n}(x)) = \lambda_{n}(\lambda(x))$. \fxnote{Notation stinks}
\end{definition}

\fxnote{iis lambda(1)(x) = x?}
To make the whole definition consistent, we have to prove that the Witt ring with the above exterior powers is indeed a $\lambda$-ring, i.e. that we indeed obtain a $\lambda$-ring homomorphism $W(R) \rightarrow W(W(R))$. \fxnote{Explain more.}

\begin{definition}
Let $R$ be a pre-$\lambda$ ring. The $k$-th \emph{Adams operation} of $R$ is the map $\gh_{k} \circ \lambda: R \rightarrow W(R) \rightarrow R$. Alternatively, let $s_{k}$ be the polynomial with $s_{k}(h_{1},h_{2},...h_{k}) = \sum\limits_{i=1}^{\infty} x_{i}^{k}$ and define $\phi_{k}(a) = s_{k}(\lambda_{1}(a),...\lambda_{k}(a))$. It follows from the above discussion that the two definitions are equivalent.
\end{definition}

\begin{prop}
Let $R$ and $S$ be two torsion-free pre-$\lambda$-rings and $f: R \rightarrow S$ any map. Then $f$ commutes with the exterior powers if and only if it commutes with the Adams operations.
\end{prop}

\begin{proof}
The only if-part is clear. For the other direction, \fxnote{Find a reference}
\end{proof}

\begin{prop}
Let $R$ be a commutative ring. Then the Adams operations of $W(R)$ with the $\lambda$-ring structure defined above are the Frobenius homomorphisms.
\end{prop}

\begin{proof}
Let $U \in \Lambda(\IZ)$ be the universal power series. Then $\phi_{n}(U)$ is $s_{n}(\lambda_{1}(U), \lambda_{2}(U), \dots)$ where $s_{n}$ is the integral polynomial with $s_{n}(h_{1}, h_{2}, \dots ) = \sum_{i} x_{i}^{n}$. Notice that $\lambda_{n}(U) = h_{n}(1-x_{1}t, 1-x_{2}t, \dots)$. \fxnote{This is confusing.}

We compute
\begin{align*}
\phi_{n}(U) &= s_{n}(\lambda_{1}(U), \lambda_{2}(U), \dots) \\
&= s_{n}(h_{1}(1-x_{1}t, 1-x_{2}t, \dots), h_{2}(1-x_{1}t, 1-x_{2}t, \dots), \dots) \\
&= \prod\limits_{i=1}^{\infty} (1-x_{i}t)^{n} \\
&= \prod\limits_{i=1}^{\infty} (1-x_{i}^{n}t) \\
&= F_{n}(U)
\end{align*}
Note that in the third line, $(1-x_{i}t)^{n}$ is the $n$-fold multiplication in the Witt ring and not the  normal power series multiplication (which is the addition in the Witt ring, whence the product in the beginning of the line, which is really a sum).  This proves the claim for the universal power series. For an arbitrary power series $p$ in a ring $R$, let $\psi: \Lambda(\IZ) \rightarrow R$ be the ring homomorphism sending $U$ to $p$. We compute
\begin{align*}
\phi_{n}(p) &= \phi_{n}(\psi(U)) \\
&= \psi(\phi_{n}(U)) \\
&= \psi(F_{n}(U)) \\
&= F_{n}(\psi(U)) \\
&= F_{n}(p)
\end{align*}
since everything is natural with respect to ring homomorphisms.
\end{proof}

\begin{prop}
The map $\lambda: W(R) \rightarrow W(W(R))$ is a ring homomorphism.
\end{prop}

\begin{proof}
If $R$ is of characteristic 0, it is easy to see that $W(R)$ is also of characteristic $0$. In this case, the ghost map $W(W(R)) \rightarrow \prod\limits_{i=1}^{\infty} W(R)$ is injective. Composing the map $\lambda: W(R) \rightarrow W(W(R))$ with the ghost map yields the ring homomorphism $\prod\limits_{i=1}^{\infty} F_{i}: W(R) \rightarrow \prod\limits_{i=1}^{\infty} W(R)$. Hence already the original map $\lambda: W(R) \rightarrow W(W(R))$  was a ring homomorphism.  If $R$ is arbitrary, pick a ring $S$ of characteristic $0$ with a surjection $S \rightarrow R$. Then also $W(S) \rightarrow W(R)$ is surjective, and everything is natural with respect to this homomorphism. A simple diagram chase yields the desired result.  
\end{proof}

\begin{prop}
The map $\lambda: W(R) \rightarrow W(W(R))$ commutes with the $\lambda$-ring structures.
\end{prop}

\begin{proof}
Again, it suffices to consider the case where $R$ is of characteristic $0$. As we have seen above, it is sufficient to prove that $\lambda$ commutes with the Adams operations, i.e. the Frobenius maps, so we have to see that $\lambda \circ F_{n} = F_{n} \circ \lambda$ (note that the left-hand Frobenius is the Frobenius of $W(R)$, whereas the other is the Frobenius of $W(W(R))$). Since $R$ has characteristic $0$, this equation can be checked in the ghost coordinates of $W(W(R))$: We have on the one hand
\[
\gh_{m}\circ \lambda \circ F_{n} = F_{m} \circ F_{n} = F_{mn}
\]
since $\gh_{m}\circ \lambda$ is the $m$-th Adams operation, and on the other hand
\[
\gh_{m} \circ F_{n} \circ \lambda = \gh_{mn} \circ \lambda = F_{mn}
\]
by the relationship of the Frobenius and ghost maps. This proves the claim.
\end{proof}

As a consequence, we obtain the following properties for arbitrary Adams operations:

\begin{prop}
Let $R$ be a $\lambda$-ring. Then the Adams operations are ring homomorphisms satisfying $\phi_{n} \circ \phi_{k} = \phi_{nk}$. Furthermore, if $\lambda_{1} = id$, as is often the case, then for all prime numbers $p$, one has $\phi_{p}(a) = a^{p} mod pA$.
\end{prop}

\begin{proof}
The Adams operations are ring homomorphisms since both $\lambda$ and $\gh_{k}$ are. Since $\lambda$ commutes with the exterior powers of $R$ and $W(R)$, it also commutes with the two sets of Adams operations. Since the Adams operations on $W(R)$ are the Frobenius maps, this means that $\lambda \circ \phi_{n} = F_{n} \circ \lambda$ and hence
$\lambda \circ \gh_{n} \circ \lambda = F_{n} \circ \lambda$. Now we compute
\begin{align*}
\phi_{n} \circ \phi_{k} &= \gh_{n} \circ \lambda \circ \gh_{k} \circ \lambda \\
&= \gh_{n} \circ F_{k} \circ \lambda \\
&= \gh_{nk} \circ \lambda \\
&= \phi_{nk} 
\end{align*}
For the final claim, write $\lambda(a) = \prod\limits_{i=1}^{\infty} (1-b_{i}t^{i})$ with $b_{1} = \lambda_{1}(a) = a$. Then we have $\phi_{p}(a) = \gh_{p} \lambda(a) = a^{p}+pb_{p}$ which proves the claim.
\end{proof}

\subsubsection{Binomial rings}

\begin{definition}
A torsion-free ring $R$ is \emph{binomial} if for all $n \in \IN$ and all $a \in R$, the element $\binom{a}{n} = \frac{a(a-1)(a-2)\dots (a-n+1)}{n!}$ of $A \otimes \IQ$ is actually in $A$.
\end{definition}

\fxnote{Some examples?}

\begin{prop}
A ring is binomial if and only if it is a torsion-free $\lambda$-ring all of whose Adams operations are the identity.
\end{prop}

\begin{proof}
First assume $R$ is binomial. Then define a map $\lambda: R \rightarrow W(R)$ by $\lambda(a) = (1-t)^{a} = \sum\limits_{i=0}^{\infty} \binom{a}{i} t^{i}$. Composing this map with the ghost map, we find
\begin{align*}
\gh \circ \lambda(a) &= -t \frac{d}{dt} \log((1-t)^{a}) \\
&= -t a \frac{d}{dt} \log(1-t) \\
&= \frac{at}{1-t} \\
&= at+at^{2}+at^{3}+...
\end{align*}
so $\gh_{n}(\lambda(a)) = a$ for all $n$. Hence $\gh \circ \lambda$ is a ring homomorphism, and since $R$ is torsion-free, this implies that $\lambda$ is a ring homomorphism.  Since $\phi_{n} = \gh_{n} \circ \lambda$, the computation also proves that all Adams operations are the identity. It remains to see that $\lambda$ commutes with the $\lambda$-ring structures. For this, it is sufficient to check that it commutes with the Adams operations. The Adams operations on $R$ are the identities, and the Adams operations on $W(R)$ are the Frobenius maps, so we have to prove that
\[
\lambda(a) = F_{n} \lambda(a)
\]
Since $R$ is torsion-free, we can check this identity in ghost coordinates. We have
\[
\gh_{k} \lambda(a) = a
\]
and
\[
\gh_{k} F_{n} \lambda(a) = \gh_{kn} \lambda(a) = a
\]
since $\gh_{i} \circ \lambda$ are the Adams operations of $R$. 
 \\
Conversely, assume $R$ is a torsion-free $\lambda$-ring all of whose Adams operations are the identity, so we have $\gh_{n}(\lambda(a)) = a$ for all $n$ and all $a \in R$. Now we compute as above in $A \otimes \IQ$ that 
\[
\gh_{n}((1-t)^{a}) = a
\]
for all $n$. Since the ghost map $\gh$ for $A \otimes \IQ$ is injective and we already have $\gh_{n}(\lambda(a)) = a$ for all $n$, where we view $\lambda(a)$ as an element of $A \otimes \IQ$, it follows that $\lambda(a) = (1-t)^{a}$ in $(A \otimes \IQ)[[t]]$; since $\lambda(a) \in A[[t]]$, we must have $(1-t)^{a} \in A[[t]]$, and this is what we wanted to prove.
\end{proof}

\begin{cor}
If $R$ is binomial, the ring $W(R)$ is an $R$-algebra.
\end{cor}

For binomial rings, we have a third possibility of expressing the ghost coordinates:

\begin{prop}
\label{binomial}
Let $R$ be a binomial ring. Then any power series $p = 1+a_{1}t+a_{2}t^{2}+ \dots$ has a unique expansion of the form $\prod\limits_{i=1}^{\infty} (1-t^{i})^{b_{i}}$. Consequently, we get a third identification of $\prod\limits_{i=1}^{\infty} R$ with $1+tR[[t]]$. With this identification, the ghost map takes the form
\[
\gh_{n}(b_{1}, b_{2}, \dots) = \sum\limits_{d \mid n} db_{d}
\]
\end{prop}

\begin{proof}
To prove the first claim, it suffices to see that the inverse of $p$ can be written as $\prod\limits_{i=1}^{\infty} (1-t^{i})^{b_{i}}$. The power series $p(1-t)^{a_{1}}$ is of the form $q = 1+b_{2}t^{2}+b_{3}t^{3}+ \cdots$. Then the power series $q(1-t^{2})^{b_{2}}$ is of the form $1+c_{3}t^{3}+c_{4}t^{4}+ \cdots$. Proceeding in this fashion, we can write the inverse of $p$ in the desired way.

  \fxnote{Continue}
\end{proof}

\subsection{Burnside ring of the infinite cyclic group and the Witt ring}

The Witt ring functor is also closely related to the Burnside ring of the integers. First, let us define the Burnside ring of a group $G$:

\begin{definition}
Let $G$ be an arbitrary group. The set of isomorphism classes of finite $G$-sets forms a monoid under the disjoint union of $G$-sets and also carries a multiplication given by the cartesian product of $G$-sets. The \emph{Burnside ring} $B(G)$ of $G$ is the Grothendieck group of this monoid, with the multiplication induced by the cartesian product.
\end{definition}

As an abelian group, $B(G)$ is quite simple: Each finite $G$-set is the disjoint union of its orbits, and the orbits are of the form $G/H$ with $H$ of finite index in G. This decomposition is unique up to conjugation of $H$, so $B(G)$ is the free abelian group with one generator for each conjugacy class of finite-index subgroups of $G$. In particular, for the infinite cyclic group $C$, the Burnside ring $B(C)$ is the free abelian group with one generator for each natural number $n$, corresponding to the subgroup $nC$. We will now concentrate on the case of $C$. The constructions we are about to make can be generalised, yielding for each group $G$ a Wittvector-like functor $W_{G}: \operatorname{CRings} \rightarrow \operatorname{CRings}$; we refer the reader to \cite{elliott} and \cite{Dress-Witt}. One may ignore the profinite-condition present in these paper by considering all subgroups instead of only the closed ones; however, the resulting functor will only depend on the profinite completion of $G$ anyway. \\
To avoid confusion, we now adopt the notation $C$ for $\IZ$ as abelian group. Given a finite $C$-set $X$, we obtain for each natural number $n$ the number of $nC$-fixed points of $X$. Since taking fixed points is compatible with coproducts and products of $C$-sets, we obtain a ring homomorphism
\[
\gh_{k}: B(C) \rightarrow \IZ
\]
The notation $\gh_{k}$ is well-chosen, as we will soon see. Let us first record the following:

\begin{prop}
If two finite $C$-sets $X$ and $Y$ have the same number of $kC$-fixed points for each $k$, they are isomorphic. 
\end{prop}

\begin{proof}
\fxnote{add}
\end{proof}

We also have operations $F_{n}$ and $V_{n}$ on $B(C)$. Again, the names are well-chosen as we will see later. The operation $F_{n}$ is obtained as follows: By restriction along the map $nC \rightarrow C$, we may view a finite $C$-set as a finite $n\IZ$-set. But since $C \cong nC$, we can view the set $X$ with the restricted action as a $C$-set again. In effect, we redefine the $C$-action on $X$ by letting $1 \in C$ act as $n$. Since restriction is compatible with products and coproducts, we obtain a ring homomorphism
\[
F_{n}: B(C) \rightarrow B(C)
\]
The operation $V_{n}$ is defined in nearly the same way with restriction replaced by induction. Explicitly, let $X$ be a finite $C$-set, which we can regard as a finite $nC$-set via the isomorphism $C \cong nC$. Then we can induce up along $nX \rightarrow C$ to obtain a new finite $C$-set $V_{n}(X)$. Induction is compatible with coproducts (though not with products), so we obtain a group homomorphism
\[
V_{n}: B(C) \rightarrow B(C)
\]

The following formula for the relationship between $\gh_{k}$, $F_{n}$ and $V_{n}$ should look familiar to the reader by now;

\begin{prop}
We have for all $n,k$
\[
\gh_{k}(F_{n}(x)) = \gh_{kn}(x)
\]
and
\[
\gh_{k}(V_{n}(x)) = \begin{cases} 
0 &\text{ if } n \nmid k \\
n \cdot \gh_{\frac{k}{n}} &\text{ if } n \mid k
\end{cases}
\]
\end{prop}

\begin{proof}
The number of $(nk)C$-fixed points of a $C$-set $X$ is the same as the number of $kC$-fixed points of $F_{n}(X)$, which proves the first claim. For the second claim, consider $X$ as an $nC$-set via the isomorphism $C \cong nC$. Then we form the induction $C \times_{nC} X$ and try to compute its $kC$-fixed points. A tuple $(c,x) \in C \times_{nC} X$ is a $kC$-fixed point if and only if $(k+c,x)$ and $(c,x)$ represent the same point of $C \times_{nC} X$. This happens if and only if $(k+c,x)$ is of the form $(c+\mu n, (-\mu)x)$ for some $\mu$ (recall that $n$ now acts as the one $1$ of $C$ on $X$, since we consider $X$ as an $nC$-set). This never happens if $n$ does not divide $k$, proving the first half of the desired formula. If $n$ divides $k$, there is a unique $\mu$ we can use, namely $\frac{k}{n}$. So in order to have $(c+\mu n, (-\mu)x = (k+c,x)$ in $C \times_{nC} X$, $x$ must be fixed under $\frac{k}{n}$. For each $x$ fixed under $\frac{k}{n}$, we now find $n$ $kC$-fixed points in $C \times_{nC} X$, namely $(0,x), (1,x),\cdots (n-1,x)$. These are all since, for example, $(n,x) = (\frac{k}{n}\cdot n, x) = (0, \frac{k}{n}x) = (0,x)$. This proves the claim.
\end{proof}

\begin{prop}
The $F_{n}$ and $V_{n}$ satisfy the following additional relations:
\begin{enumerate}
\item $F_{n} \circ V_{n}$ is multiplication with $n$.
\item $F_{m} \circ F_{n} = F_{mn}$
\item $V_{m} \circ F_{n} = F_{n} \circ V_{m}$ if $gcd(m,n) = 1$.
\item $F_{m}$ is a ring homomorphism.
\item $V_{m}(a * F_{m}(b)) = (V_{m}(a)) * b$ where $*$ is the multiplication in the Burnside ring.
\end{enumerate}
\end{prop}

\begin{proof}
All of these equations boil down to formulas about induction and restriction. The last one is the Frobenius reciprocity formula. We leave it to the reader to work out the details.
\end{proof}

Our notation already heavily suggests that there is a relationship between the Burnside ring and Witt vectors, and indeed we have the following:

\begin{prop}
The group homomorphism $B(C) \rightarrow 1+t\IZ[[t]]$ given by $nC \mapsto 1-t^{n}$ on generators is a ring injection from $B(C)$ to $W(R)$. Under this ring injection, the two ghost, Frobenius respectively Verschiebung maps correspond to each other. 
\end{prop}

\begin{proof}
Starting with a $C$-set $X$, consider the free $\IZ$-module with basis $X$ $\IZ(X)$. This $\IZ$-module has a canonical automorphism $f(X)$ given on the basis by sending $x$ to $1x$, which we can also view as an endomorphism of $\IZ(X)$. It is straightforward to check that this gives a ring homomorphism $B(C) \rightarrow \End_{0}(\IZ)$. To check multiplicativity, note that $f(X) \otimes f(Y)$ corresponds to $f(X \times Y)$ under the canonical isomorphism $\IZ(X) \otimes \IZ(Y) \cong Z(X \times Y)$. It is also straightforward to see that composing this map with the characteristic polynomial-map $\End_{0}(\IZ) \rightarrow W(R)$ gives the map described in the proposition. So it suffices to see that $B(C) \rightarrow \End_{0}(\IZ)$ is injective and compatible with ghost, Frobenius and Verschiebung maps. Injectivity follows because both rings are torsion-free and the polynomials $1-t^{n}$ are linearly independent. To see the other claims, note that for a $C$-set $X$, the objects $(\IZ(X), f(X)^{n})$ and $(\IZ(\res_{nC}^{C}(X)), f(\res_{nC}^{C}(X)))$ of the endomorphism category are isomorphic - this is more or less a tautology once one goes through the definitions. With this, the necessary calculation for the ghost maps is easy, and the claim for Frobenius and Verschiebung follow from this since the two possible Frobenius and Verschiebung maps have the same behaviour under the ghost map.
\end{proof}

\fxnote{Continue: almost finite C-sets}

%\subsection{Some combinatorics}

%\begin{prop}
%Let $p$ be a prime number, $\IF_{p}$ the field with $p$ elements and $a_{i} \in \IN$ the number of irreducible monic polynomials of degree $i$ over $\IF_{p}$. The sequence $a_{i}$ satisfies 
%\[
%\sum\limits_{d \mid n} da_{d} = p^{n}
%\]
%\end{prop}

%\begin{proof}
%add
%\end{proof}

%\subsection{Generalizing to arbitrary groups}

%dadada

\cite{alm-endo}
\cite{alm-trace}
\cite{BLR}
\cite{Lance}
\cite{Swan}
\cite{KThandbook}
\cite{coefficients}
\cite{elliott}
\end{appendix}
