# Supplementary material for: The Baum-Connes conjecture, Swan group actions and controlled topology
Source: arXiv:1303.0701 source file (2013-03-04)
Supplement: Supplementary file 2 [file appendix2.tex]

\begin{appendix}

\chapter{Appendix}
\section{$C^{*}$-algebras and continuous function calculus}

This section is a short reminder of the definition of the continuous function calculus on a $C^{*}$-algebra. \\

\begin{definition}
For a commutative $C^{*}$-algebra $A$, let $Sp(A)$ be the set of algebra homomorphisms from $A$ to $\IC$. We view $Sp(A)$ as a subspace of the space of linear functionals $A \rightarrow \IC$, equipped with the weak-$^{*}$-topology.
\end{definition}

\fxnote{define U(A) and GL(A) for nonunital algebras}

\begin{prop}
\label{unitaryvsinvertible}
Let $A$ be a $C^{*}-algebra$. Then $U(A)$ is a deformation retract of $GL(A)$.
\end{prop}

\begin{proof}
Let us first consider the case where $A$ already is unital. Then $U(A)$ and $GL(A)$ are just the unitaries respectively invertibles in $A$. Let $x$ be invertible. Then %find source
\end{proof}

\pagebreak
\section{Hilbert Modules}

\begin{example}
Let $A$ be a $C^{*}$-algebra and $a_{1}, a_{2}, \cdots$ a sequence of elements of norm $1$. Then the matrix
\[
\begin{pmatrix}
a_{1} \\
a_{2} \\
a_{3} \\
\cdots
\end{pmatrix}
\]
never represents a bounded operator from $A$ to $\oplus_{\IN} A$. However, its potential adjoint
\[
\begin{pmatrix}
a_{1} & a_{2} & a_{3} & \cdots
\end{pmatrix}
\]
may represent a bounded operator. For example, if $A = C[0,1]$, let $a_{i}$ be a continuous function supported on $[\frac{1}{i+1}, \frac{1}{i}]$ with norm $1$. Then we estimate for the corresponding operator $T: \oplus_{\IN} A \rightarrow A$
\begin{align*}
\left\Vert T(\sum\limits_{\IN} b_{i} e_{i}) \right\Vert^{2} 
&= \left\Vert \sum\limits_{\IN} b_{i} a_{i}  \right\Vert^{2} \\
&= \sup_{i} \left\Vert b_{i} \right\Vert^{2} \\
&\leq \left\Vert \sum\limits_{\IN} b_{i}b_{i}^{*} \right\Vert \\
&= \left\Vert \sum\limits_{\IN} b_{i}e_{i} \right\Vert
\end{align*}
and hence $T$ is bounded. \fxnote{Check.}
\end{example}

\pagebreak
\section{Crossed products}

This section collects some definitions and facts about twisted group rings and reduced crossed products. 

\begin{definition}
Let $A$ be a ring with a left $G$-action, which we will denote by $(a,g) \mapsto g(a)$. The twisted group ring or crossed product of $A$ and $G$ $A \rtimes G$ is the ring with elements formal finite sums $\sum\limits_{i} a_{i} g_{i}$ with $g_{i} \in G, a_{i} \in A$. Multiplication is defined by setting
\[
ag \cdot bh = a g(b) gh
\]
and extending $\IZ$-bilinearly. It is easy to check that this multiplication is associative.
\end{definition}

\begin{rem}
Analogously, we can define a twisted group ring $G \rtimes A$ if $A$ has a right $G$-action. Its elements are of the form $\sum\limits_{i} g_{i}a_{i}$, and multiplication is defined such that
\[
ga \cdot hb = gh a^{h}b
\]
Regarding a ring with right $G$-action as a ring with left $G$-action by letting $g$ act as $g^{-1}$ from the right, we can form two twisted group rings $A \rtimes G$ and $G \rtimes A$. The map sending $ga \in A \rtimes G$ to $g(a) g = (a^{g^{-1}}) g \in G \rtimes A$ is an isomorphism between these two rings.
\end{rem}

\begin{prop}
\label{covariant}
Let $M$ be a left $A$-module. A left $A \rtimes G$-module structure is then the same as a left $G$-action on $M$, $(m,g) \mapsto g(m)$ such that
\[
g(ma) = g(m)g(a)
\]
We call a pair consisting of the left actions of $A$ and $G$ satisfying this condition a covariant representation of $(A,G)$.
\end{prop}

\begin{proof}
For $ag \in G \rtimes A$, we define
\[
ag \cdot m = ag(m)
\]
and extend linearly. The only thing to check is that
\[
bh \cdot (ag \cdot m) = (bh \cdot ag) \cdot m 
\]
for $g,h \in G, a, b \in A$. The left-hand side computes to $b h(ag(m))$ and the right-hand side to $bh(a) (hg)(m)$. The assumption guarantees that this is the same.
\end{proof}

If $A$ comes with an involution and $G$ acts involution-preserving on $A$, we can define an involution on $G \rtimes A$ via
\[
(ag)^{*} = g^{-1}(a^{*}) g^{-1}
\]
It is straightforward to check that this involution is anti-multiplicative. 

\subsection{Reduced Group $C^{*}$-algebras}

Now assume $A$ is a $C^{*}$-algebra with an involution-preserving right $G$-action. 

\begin{definition}
Let $l^{2}(G,A)$ be the complete Hilbert $A$-module with basis $G$. We define a left $G$-action $\rho$ on $l^{2}(G,A)$ via
\[
\rho(g)(\sum a_{i}g_{i}) = \sum a_{i} gg_{i}
\]
and a left module action $\tau$ of $A$ on $l^{2}(G,A)$ via
\[
\tau(a)(\sum a_{i}g_{i}) = \sum g_{i}^{-1}(a)a_{i} g_{i}
\]
This is a covariant representation of $(A,G)$, called the regular representation, compare \cite[Def. 2.20]{HG}.
\end{definition}

\pagebreak
\section{$C^*$-categories and $L$-theory}

\subsection{$C^*$-algebras and symmetric forms}

The following theorem classifies symmetric forms over $C^*$-algebras; compare \cite{analyticnovikov}[1.6].

\begin{thm}
\label{forms}
Let $A$ be a $C^*$-algebra with unit and let $(A^n,p)$ be a projective module defined by a projection $p$. Let $\phi: (A^n,p) \rightarrow (A^n,p)$ be a symmetric form, i.e. a selfadjoint invertible. Then there are projections $p_+$ and $p_-$ in $A^n$ with $(A^n,p_+) \oplus (A^n,p_-) \cong (A^n,p)$ such that $\phi$ is isometric to the form $1 \oplus -1$ on $(A^n,p_+) \oplus (A^n,p_-)$, and this decomposition is unique up to isomorphism.
\end{thm}

\begin{proof}
We may assume that $\phi: A \rightarrow A$ by replacing $A$ with $\End(A^n,p)$ if necessary. If $\phi$ is positive, $\phi^{\frac{1}{2}}$ defines an isometry from $\phi$ to $1$; similarly if $\phi$ is negative, $(-\phi)^{1/2}$ defines an isometry from $\phi$ to $-1$. In general, since $\phi$ is invertible, its spectrum has a gap around $0$. Let $f_+$ be a continuous function which is $1$ on the positive part of the spectrum and $0$ on the negative part; $p_+ = f_+(\phi)$ is called the \emph{positive projection} of $\phi$. Similarly, using a function $f_-$ which is $1$ on the negative part of the spectrum and $0$ on the positive part, one defines a projection $p_-$, called the \emph{negative projection} of $\phi$.  Note that $p_+ + p_1 = 1$, hence $A \cong (A.p_+) \oplus (A,p_-)$. This splitting is $\phi$-invariant since $\phi$ commutes with both $p_+$ and $p_-$. Furthermore, $ap_+\phi = ap_+(p_+\phi)$, hence $\phi$ is given by the positive element $p_+\phi$ on $(A,p_+)$ and similarly by the negative element $p_-\phi$ on $(A,p_-)$. Hence $\phi$ decomposes as a direct sum of one negative and one positive symmetric, and we have already seen that a positive symmetric form is isometric to $1$ and a negative form is isometric to $-1$.  This proves the existence part.  \\
Proving uniqueness is unfortunately quite a mess. We have to see that, given 4 projective modules $P_1, P_2, Q_1, Q_2$ and an isometry $k$ between the two forms $1 \oplus -1: P_1 \oplus P_2$ and $1 \oplus -1: Q_1 \oplus Q_2$, $P_1$ and $Q_1$ and $P_2$ and $Q_2$ are isomorphic. Writing $k$ as a $2 \times 2$-matrix $(k_{ij})$ and writing out what it means to be an isometry between the two forms, we find that $k_{11}k_{11}^* = 1+k_{12}k_{12}^*$ and, by considering $k^*$ as an isometry in the other direction, $k_{11}^*k_{11} = 1+k_{12}^*k_{12}$ and hence $k_{11}^*k_{11}$ and $k_{11}k_{11}^*$ are both invertible. It follows that $k_{11}$ is invertible since it has both a right and a left inverse. The same argument applies to $k_{22}$.
\end{proof}

We also record a kind of "homotopy invariance" of symmetric forms:

\begin{prop}
\label{homotopy}
Let $\phi$ and $\psi$ be symmetric forms in a $C^*$-algebra $A$. Assume that $\phi$ and $\psi$ are connected by a path of selfadjoint invertibles.. Then $\phi$ and $\psi$ are isometric. By considering the linear path from $\phi$ to $\psi$, this is in particular the case if $\psi$ lies inside some open ball around $\phi$ consisting only of invertibles.
\end{prop}

\begin{proof}
Let $\gamma$ be such a path from $\phi$ to $\psi$. The process of forming the positive and negative projections of $\gamma(t)$ depends continuously on $t$, hence $\phi_+$ and $\psi_+$ are connected by a path of projections which implies that $\phi_+$ and $\psi_+$ are unitarily equivalent. The same argument applies to the negative projections, hence the proposition follows.
\end{proof}

Now that we know that isometry classes of symmetric forms on projective modules over a $C^*$-algebra correspond to pairs of isomorphism classes of projective modules, it is easy to deduce what $L_0^p$ of a $C^*$-algebra is:

\begin{prop}
The functors $K_0^{top}$ and $L_0^p$ on the category of $C^*$-algebras are naturally isomorphic.
\end{prop}

\begin{proof}
Isometry classes of symmetric forms correspond to pairs of projective modules; since 2 is invertible, dividing out hyperbolic forms corresponds to dividing out the pairs $(P,P)$ for any projective module $P$. The result is clearly $K_0^{top}$.
\end{proof}

\subsection{$C^*$-categories and symmetric forms}

The above proposition carries over to $C^*$-categories with virtually the same proof:

\begin{prop}
The functors $L_0^p$ and $K_0^{top}$ on the category of $C^*$-categories are naturally isomorphic. 
\end{prop}

\begin{proof}
Let $\phi: (A,p) \rightarrow (A,p)$ be a symmetric form. By applying \ref{forms} to the $C^*$-algebra $\End((A,p))$, we obtain projective modules $(A,p_+)$ and $(A,p_-)$ such that $\phi$ is isometric to $1 \oplus -1$ on $(A,p_+) \oplus (A,p_-)$. As above, the map $L_0^p(\C) \rightarrow K^{top}(\C), [\phi] \rightarrow p_+-p_-$, is an isomorphism.
\end{proof}

\begin{prop}
For any $C^*$-category $\C$, multiplication by $2$ annihilates both the kernel and the cokernel of the natural map $i: L_0(\C) \rightarrow L_0^p{\C}$. 
\end{prop}

\begin{proof}
This is a consequence of the Rothenberg sequence. However, since we understand symmetric forms in $C^*$-categories, we can give an explicit proof, compare \cite{analyticnovikov}[1.7]. \\
Let $\tilde{K_0}(\C)$ be the cokernel of the inclusion $K_0^{alg}(A) \rightarrow K_0^{alg}(\Idem(A))$. It easily follows from the classification of forms that $L_0(\C)$ is the group
\[
\{(P,Q) \in K_0(\Idem(\C)) \times K_0(\Idem(\C)): P+Q = 0 \in \tilde{K_0}(\C) \} / <\{(A,A): A \in \C\}>
\]

The kernel of $i$ is given by pairs $(P,P)$ in $K_0^p(\C)$ with $2P = 0$ in $\tilde{K_0}(\C)$. We may change $(P,P)$ by adding or subtracting $(A,A)$ for $A$ an actual object of $\C$ without changing the $L_0$-class $(P,P)$ represents. This means that the $L_0$-class $(P,P)$ represents only depends on $P \in \tilde{K_0}(\C)$, and hence the kernel identifies with the $2$-torsion in $\tilde{K_0}(\C)$. \\
For the cokernel, clearly $i$ hits $K_0^{alg}(\C) \subset K_0^{top}(\C) \cong L_0^p(\C)$. Hence to compute the cokernel, we may interpret $i$ as a map from $L_0(\C)$ to $\tilde{K_0}(\C)$. The image consists of the differences $P-Q$ such that $P+Q = 0$, i.e. of the elements of the form $2P$. So the cokernel is $\tilde{K_0}(\C)/2\tilde{K_0}(\C)$.
\end{proof}

\pagebreak

\end{appendix}
